# Supplementary material for: NEAT: A Label Noise-resistant Complementary Item Recommender System with Trustworthy Evaluation
Source: arXiv:2202.05456 source file (2022-02-11)
Supplement: Supplementary file 1 [file appendix.tex]

\section{Visualization of Personalized Type Representations}
We compute the personalized type representations for two users in INS respectively by Equation \ref{eq:personalized-mean} in Section 4.1 and visualize the personalized types (aisles) for each department in Figure \ref{fig:user-1} and \ref{fig:user-2} via t-SNE\cite{maaten2008visualizing} dimension-reduction.
To cover different domains of shopping scenarios, we select \texttt{Skin Care} from personal care, \texttt{Coffee} from beverage and \texttt{Condiments} from pantry as query product-types.
We plot the top-5 complementary types (annotated in black) of query types (annotated in red) with dotted lines between each pair of query type and complement type.
As we can see, our personalized type representations automatically organize around different departments (markers with same color and shape) group together.
Moreover, complementarity between types under intended functionality for users is also visualized.
Each query type recall different top-5 complementary types for two users.
% For example, when user 1 looks at \texttt{Skin Care}, the potential complementary recommendations for \texttt{Skin Care} might be under the combined topics of baby and personal care, while user 2 might be more interested in the complementary recommendations under the topics of beauty and home fragrance. 
This indicates the distinct intended functionality for two users when showing complementary recommendations.
% By doing so, we can infer the potential topics of complementary items for each user with our personalized projections of product-types and achieve topic disambiguation.

\begin{figure}[t]
    \centering
    \caption{Personalized Type Representations for User 1.}
    \includegraphics[width=\linewidth]{image/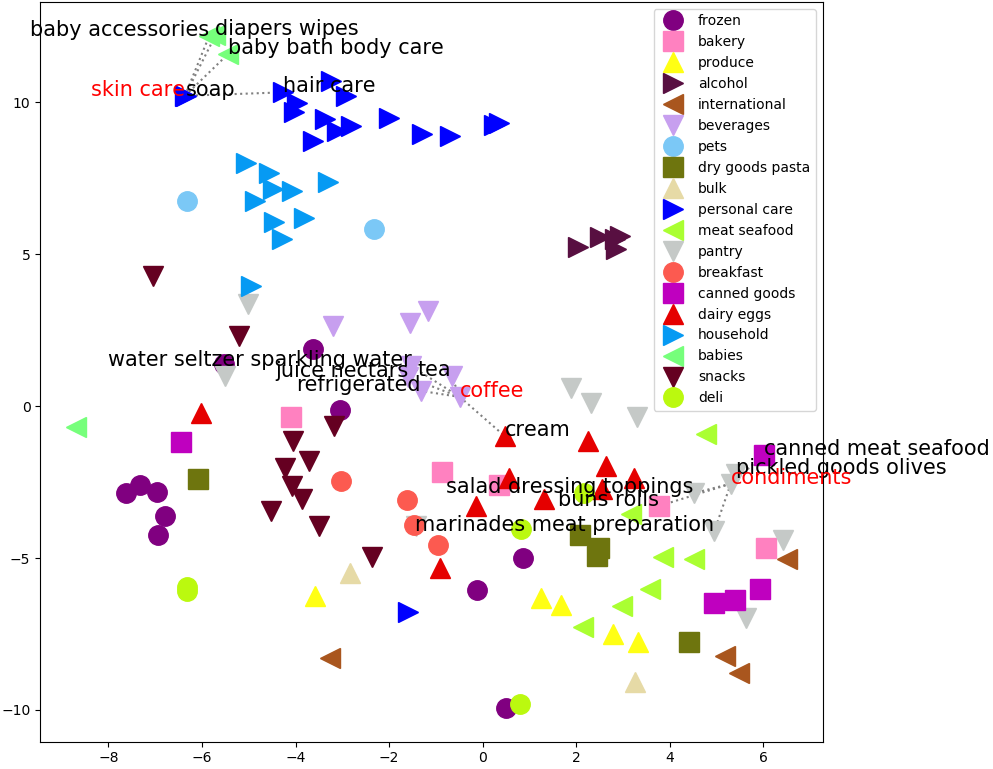}
    \label{fig:user-1}
\end{figure}
\begin{figure}[b]
    \centering
    \caption{Personalized Type Representations for User 2.}
    \includegraphics[width=\linewidth]{image/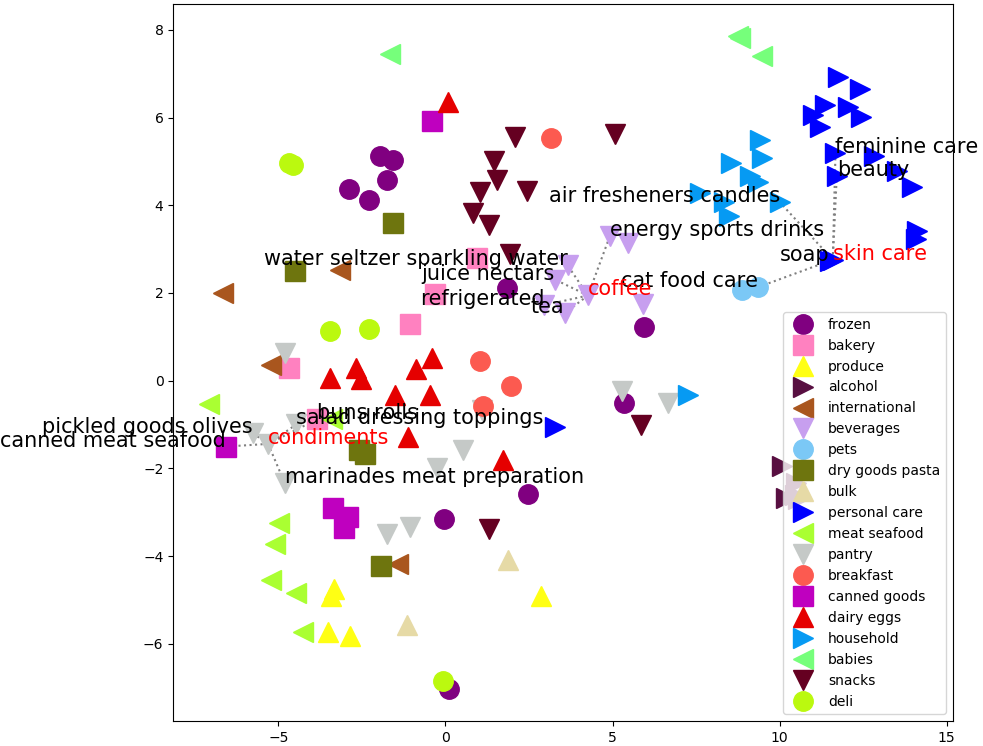}
    \label{fig:user-2}
\end{figure}
% \begin{figure}
%     \centering
%     \caption{Personalized projection of product-types for User 1 \& 2 in Instacart dataset, with query product-types (annotated in red) and their top-5 nearest neighbors (annotated in black).}
%     \begin{subfigure}[b]{\linewidth}
%         \centering
%         \caption{Personalized projection of product-types for User 1.}
%     \includegraphics[width=\linewidth]{image/random_user1_small.png}
%     \label{fig:user-1}
%     \end{subfigure}\hfill
%     \begin{subfigure}[b]{\linewidth}
%         \centering
%         \caption{Personalized projection of product-types for User 2.}
%     \includegraphics[width=\linewidth]{image/random_user2_small.png}
%     \label{fig:user-2}
%     \end{subfigure}
% \end{figure}
